# Supplementary material for: Spin-polarizing electron beam splitter from crossed graphene nanoribbons
Source: arXiv:2201.07147 source file (2022-07-12)
Supplement: Supplementary file 1 [file supp-info.pdf]

# Supplementary material:
# A spin-polarizing electron beam splitter from crossed graphene nanoribbons

Sofia Sanz,[1,*] Nick Papior,[2] Géza Giedke,[1,3] Daniel Sánchez-Portal,[4] Mads Brandbyge,[5,6] and Thomas Frederiksen[1,3,†]

[1] *Donostia International Physics Center (DIPC), E-20018, Donostia-San Sebastián, Spain*

[2] *DTU Computing Center, Technical University of Denmark, DK-2800 Kgs. Lyngby, Denmark*

[3] *IKERBASQUE, Basque Foundation for Science, E-48013, Bilbao, Spain*

[4] *Centro de Física de Materiales (CFM) CSIC-UPV/EHU, E-20018, Donostia-San Sebastián, Spain*

[5] *Department of Physics, Technical University of Denmark, DK-2800 Kgs. Lyngby, Denmark*

[6] *Center for Nanostructured Graphene (CNG), Denmark*

(Dated: July 12, 2022)

## SUMMARY OF CONTENT

In this supplementary material we describe our methodology and present additional calculations that may be interesting for a deeper understanding of the reported effects. In Sec. S1 we explain the details of the calculation with the mean-field Hubbard model (MFH). In Sec. S2 we show the effect of the Coulomb repulsion on the bands of bilayer and monolayer graphene nanoribbons, while in Sec. S3 we show the effect that the size of the scattering region has on the local magnetization of the device. Next in Sec. S4 we plot all the possible spin configurations resulting from the possible combinations of the spin densities of the four electrodes. In Secs. S6 and S7 we show the figure of merit, where we analyze the quality of the device as a spin-beam splitter or mirror, and the spin polarization at a different electronic energy from the one shown in the main text, respectively. In Sec. S8 we compare the transport properties for different ribbon widths. In Sec. S9 we show the quality of the independent scatterers approximation compared to the exact result for a device with three crossings. In Sec. S10 we compare the spin-averaged transmission probabilities with the unpolarized case. In Sec. S11 we explore how possible distortions, such as a small twist angle or a lateral translation of the on-top ribbon with respect to the bottom one, affect the transport properties of individual crossings. In Sec. S12 we describe the used statistical sampling and analytical expression for the averaged spin-polarization shown in Fig. 4(b) of the main text. Finally, in Sec. S13 we analyze the spin-polarizing beam-splitting effect that can be found in junctions formed with other edge-polarized GNRs, such as those built with crossed bearded GNRs.

* sofia.sanz@dipc.org
† thomas_frederiksen@ehu.eus

**CONTENTS**


Summary of content 2

S1. Solving the MFH with open boundary conditions 4

S2. Effect of $U$ in the band structure of mono- and bilayer ZGNRs 7

S3. Distance from the scattering center to the electrodes 10

S4. All inequivalent spin configurations and transmission curves for AB- and AA-stackings 12

S5. Electronic total energy and magnetization 17

S6. Figure of merit 19

S7. Spin polarization for electrons at other energy values 20

S8. Role of ribbon width 22

S9. Independent-scatterers approximation 23

S10. Averaged transmission probabilities 25

S11. Role of crossing geometry for the spin-polarizing transport effect 27

S12. Statistical analysis of random array devices 29

S13. A spin-polarizing beam splitter with bearded GNRs 34

References 37

## S1. SOLVING THE MFH WITH OPEN BOUNDARY CONDITIONS

The Hubbard Hamiltonian in the mean-field approximation model has proven to be in remarkable agreement with quantum Monte Carlo simulations for ZGNR for moderate Coulomb interactions [1]. The complete geometry is divided into the relevant parts here involved: the semi-infinite electrodes and the scattering area (device), where the latter contains the crossing between the two infinite ribbons, $H_T = H_d + \sum_\alpha (H_\alpha + H_{\alpha d})$, where $H_d$ is the device Hamiltonian and $H_\alpha, H_{\alpha d}$ are the $\alpha$th electrode Hamiltonian and its coupling to the device region. The occupation of the electronic states is defined by Fermi-Dirac statistics with a temperature set to $T = 300$ K. For our system the band gap opening is of the order 500 meV, *i.e.*, $\sim 25 \times kT$ at this temperature (and $k$ the Boltzmann constant), which implies that the distribution function is basically a step function. Therefore, practically there is no difference with the results one would obtain at lower temperatures. We also assume an orthogonal basis of localized atomic orbitals. Further, the qualitative picture presented in the main text is not affected by the numerical choice for the Coulomb repulsion parameter $U = 3$ eV, but only the quantitative results. To show this last statement we have calculated the transmission probabilities for the $\boxed{\uparrow\uparrow}$ device obtained with $U = 1.5$ eV in Fig. S1.

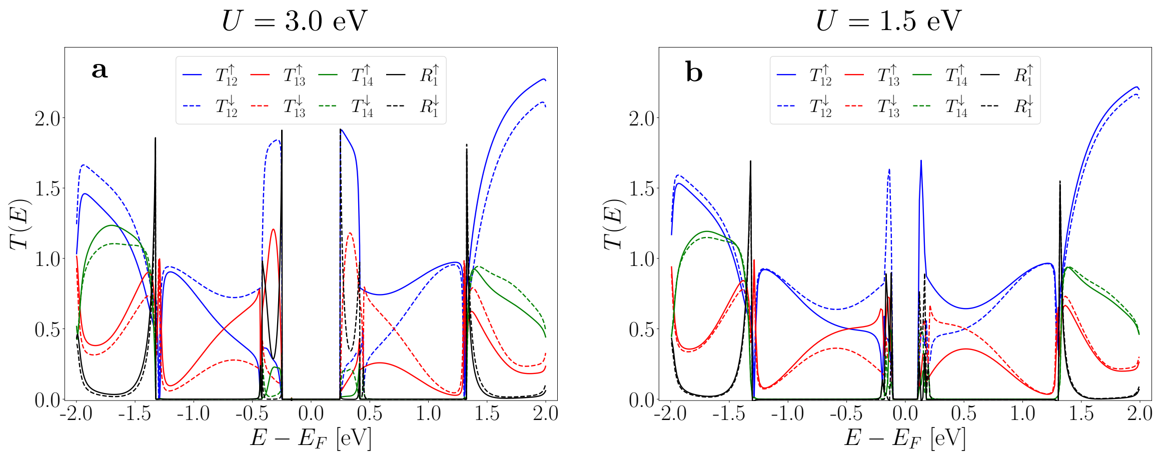


FIG. S1. Transmission probability for an incoming electron from terminal 1 of the $\boxed{\uparrow\uparrow}$ device obtained with (a) $U = 3$ eV and (b) $U = 1.5$ eV.

The computational setup begins by solving the electrodes, where the spin densities $\langle n_{i,\sigma} \rangle$ are found by diagonalization of the infinite ZGNR's unit-cell at each $\mathbf{k}$-point over the Brillouin zone. The spin-densities will be used to update the Hamiltonian of Eq. (1) in each

iteration, until the convergence criterion is achieved, as implemented in our PYTHON package HUBBARD [2]. To properly account for the effect of the semi-infinite leads in the device Hamiltonian, the spin densities in equilibrium are computed by an integration of the Green's function along a predefined energy contour in the complex plane [3] that we obtained from TRANSIESTA [4],

$$\langle n_{i,\sigma}\rangle = \frac{1}{2\pi}\left[\int_{-\infty}^{\infty}\mathbf{A}_\sigma(\varepsilon)n_F(\varepsilon-\mu)d\varepsilon\right]_{ii}, \tag{S1}$$

where $n_F(\varepsilon-\mu)$ is the Fermi distribution with $\mu$ the electrochemical potential, $\mathbf{A}_\sigma = i\left(\mathbf{G}_\sigma - \mathbf{G}_\sigma^\dagger\right)$ is the spectral function and $\mathbf{G}_\sigma^{-1} = (\varepsilon + i\eta)\mathbf{I} - \mathbf{H}_{C,\sigma} - \sum_\alpha \mathbf{\Sigma}_{\alpha,\sigma}$ is the retarded Green's function for each spin component $\sigma$. $\mathbf{\Sigma}_{\alpha,\sigma}$ is the self-energy matrix that accounts for the coupling between the $\alpha$th semi-infinite lead with spin component $\sigma$ to the scattering region. The self-energy matrices are converged with the Lopez-Sancho recursive method [5] as implemented in the open source, Python-based SISL package [4, 6] using a small broadening of $\eta = 1$ meV. For clarification, the flow diagram of the self-consistent cycle is plotted in Fig. S2.

For equilibrium calculations the electronic contribution to the total energy can be calculated as

$$E_{\text{tot}} = \sum_{\sigma=\uparrow,\downarrow}\frac{1}{2\pi}\int \text{Tr}\left[\mathbf{A}_\sigma(\varepsilon)\right]n_F(\varepsilon-\mu)\varepsilon d\varepsilon - U\langle n_\uparrow\rangle\langle n_\downarrow\rangle, \tag{S2}$$

where the left term of Eq. (S2) is the integration of the occupied states while the right term comes from the interaction term of the Hamiltonian. To perform the numerical transport calculations we have used the free and open-source code TBTRANS [4].

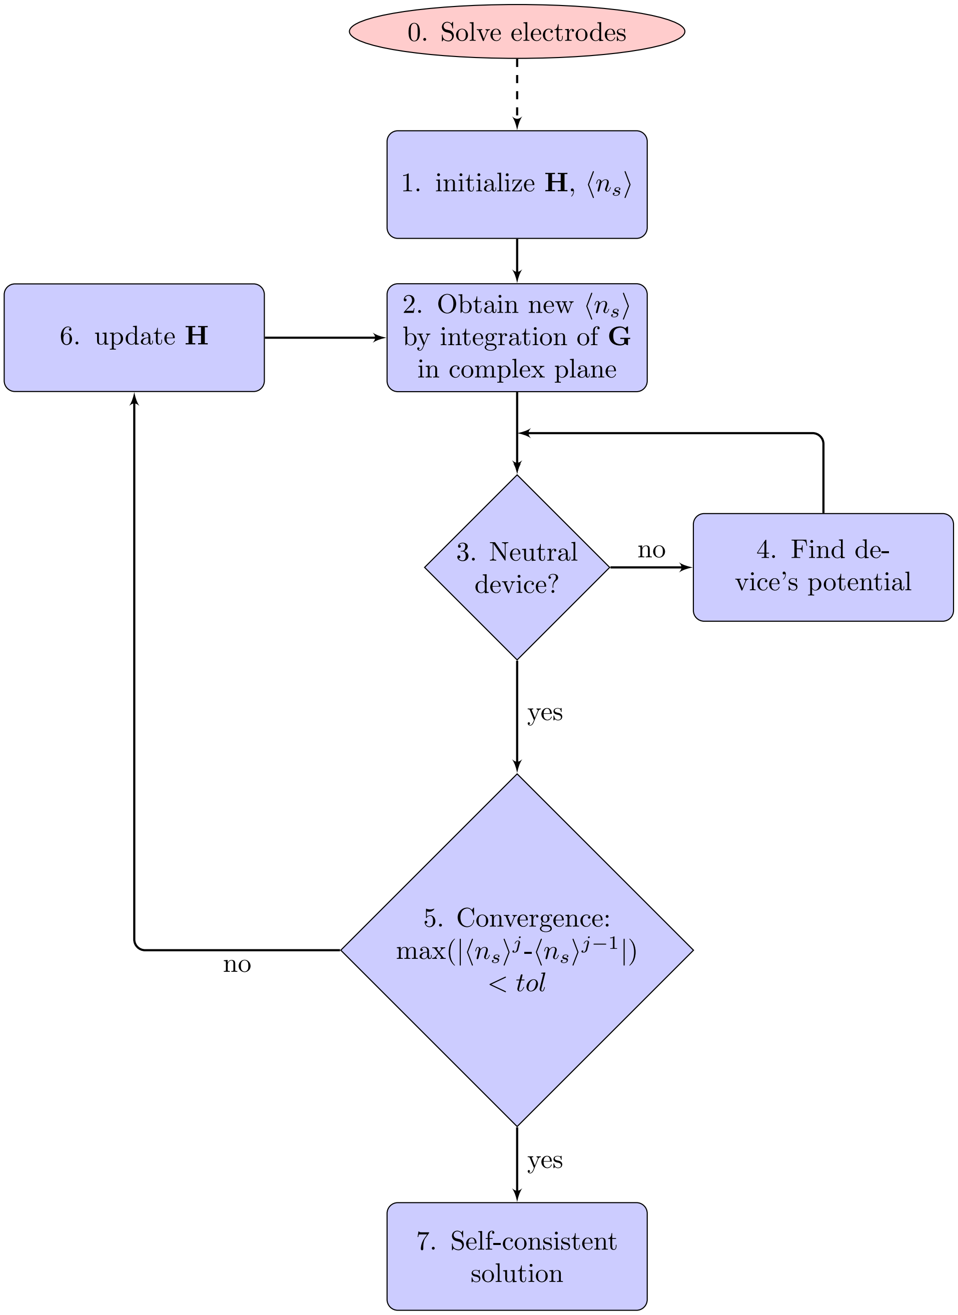


FIG. S2. Convergence process of the MFH model with open boundary conditions.

## S2. EFFECT OF $U$ IN THE BAND STRUCTURE OF MONO- AND BILAYER ZGNRS

In this section we show the band structures for periodic mono- and bilayer $w$-ZGNRs for widths of $w = 8, 16$ carbon atoms across. The geometries of the AA- and AB-stacked ZGNRs are shown in Fig. S3(a,b). In Fig. S3(c-h) we show the band structures for the unpolarized (black dashed lines) and polarized (color lines) Hamiltonians with $U = 3$ eV. The main effect of the interaction term on the electronic structures of these systems is the opening of the correlation gap around $E_F$. While the larger hybridization in the AA-stacking pushes the edge states further in energy for the unpolarized case (panels (e,f)), which competes with the Coulomb repulsion parameter, in the AB-stacking case the presence of the flat bands (edge states) give rise to the opening of a correlation gap around $E_F$. The spin distribution of the bilayer ZGNRs (of lowest energy) is composed of two polarized monolayer ZGNRs (antiferromagnetic alignment between the edges of the ribbons) while the atoms that are vertically aligned are also antiferromagnetically aligned. These results are in line with DFT calculations [7].

In Fig. S4 we plot the polarization represented by the center of mass of the wavefunctions $\psi^{\uparrow}_{n\mathbf{k}}$, calculated as $\int y|\psi^{\uparrow}_{n\mathbf{k}}|^2 dy$, for the case of the monolayer 8-ZGNR. For an unpolarized wave the center of mass of the wave coincides with the geometrical center of the unit cell, given the inversion symmetry of the ZGNR unit cell. However, for the polarized ZGNR, this is not necessarily the case given the symmetry breaking between the two spin components.

We observe a large polarization of the wave especially in the valence and conduction bands. We also find an interesting behavior of the spin-wave distribution, where the center of mass of the wave transitions from the lower half of the unit cell to the upper half as $k$ goes from $\Gamma$ to X. This explains the spin majority on the different sublattices depending on the electron energy.

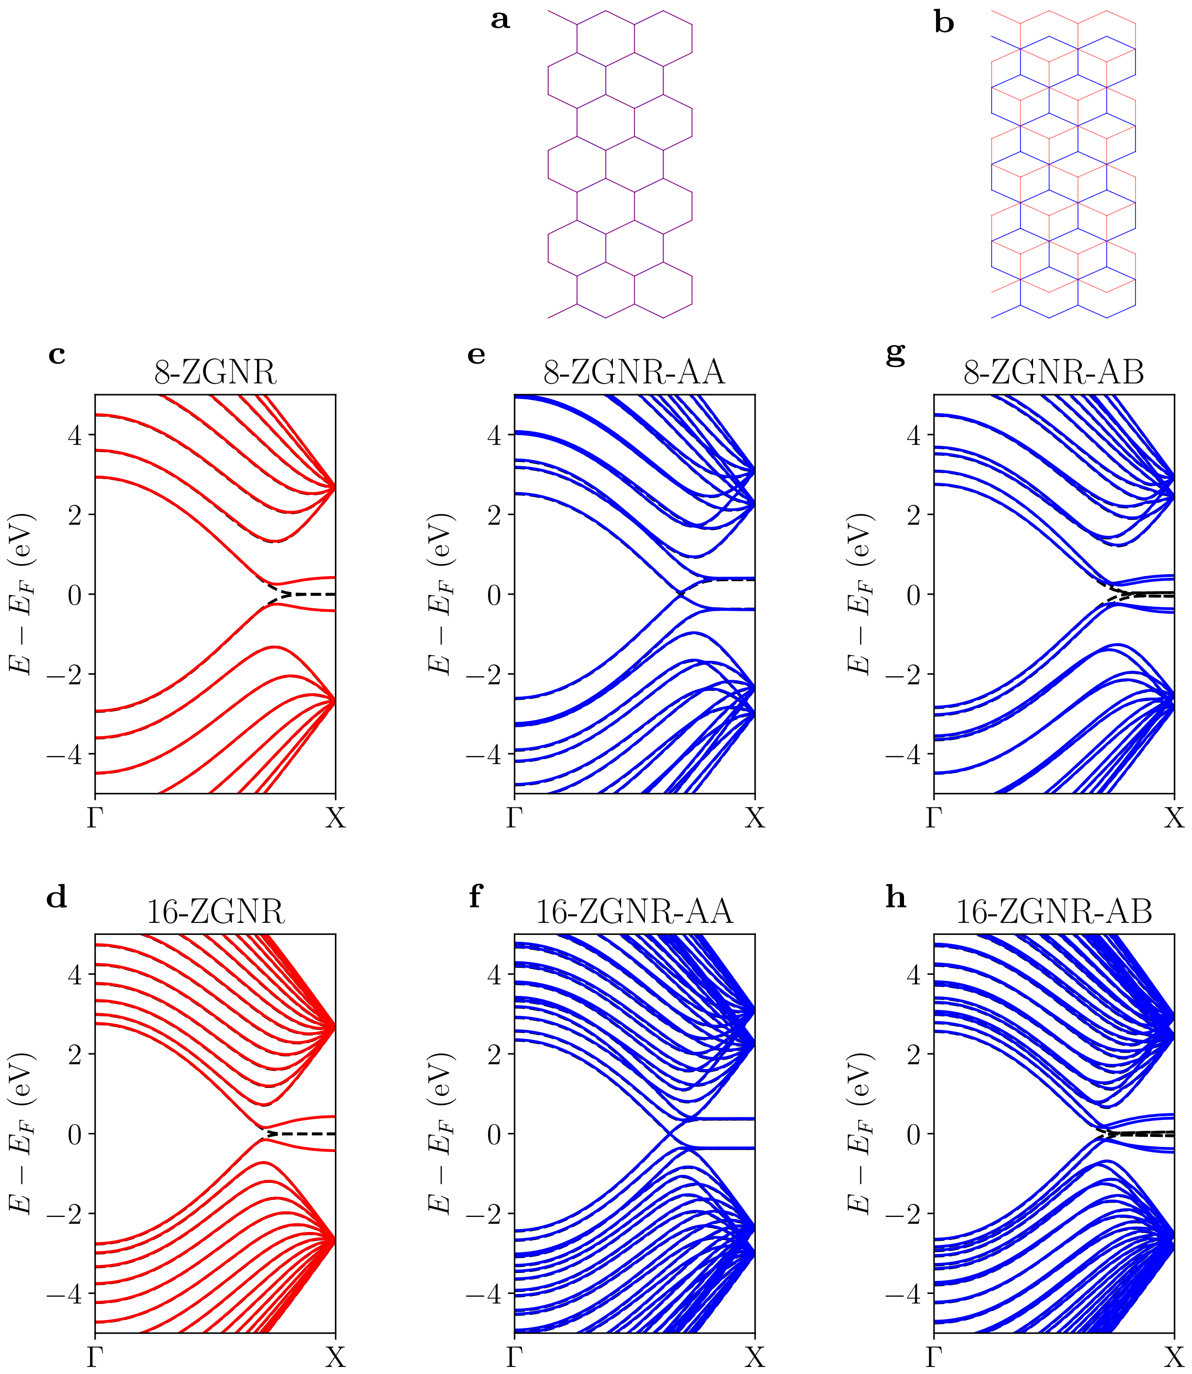


FIG. S3. Band structures of mono- and bilayer $w$-ZGNRs of different widths. (a,b) Geometry of the AA- and AB-stacked bilayer 8-ZGNRs. Band structure along the Γ–X path for (c,d) monolayer and (e,f) bilayer AA-stacked and (g,h) bilayer AB-stacked 8-ZGNRs. Black dashed lines show the band structures for $U = 0$ and colored lines those obtained after convergence with $U = 3$ eV.

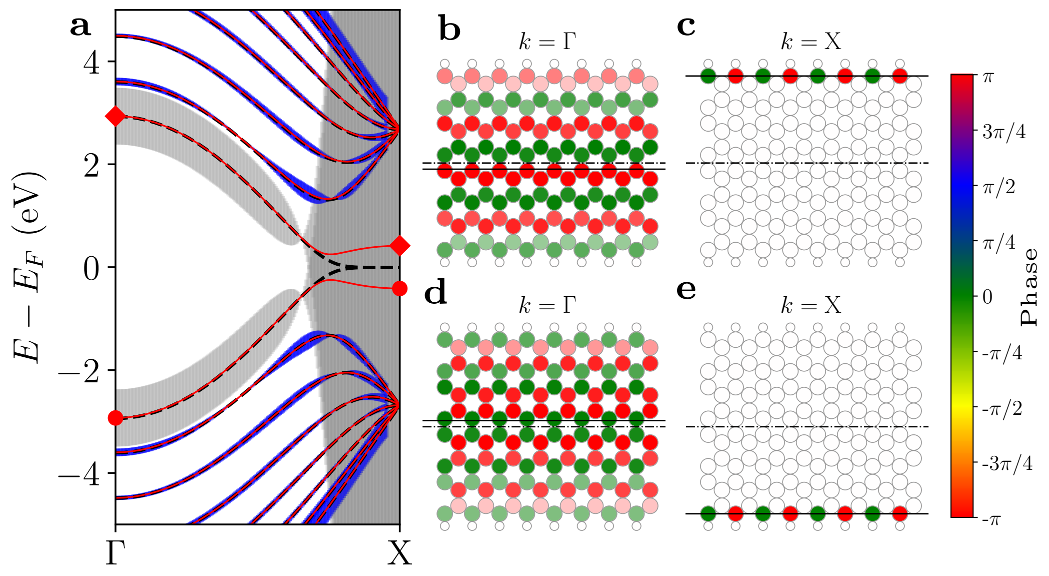


FIG. S4. (a) Band structure for the periodic unpolarized (black dashed lines) and polarized (red solid lines) 8-ZGNR. We also show the position of the center of mass of the wave functions $\psi^{\uparrow}_{n\mathbf{k}}$ plotted as a "fat-band" analysis, where the size of the error bars is computed as $\left|\int y|\psi^{\uparrow}_{n\mathbf{k}}|^2 dy\right|$. We plot the fat-bands in grey for the valence and conduction bands and blue for the remaining bands. (b,c) Spatial distribution of the Bloch wave functions $\psi^{\uparrow}_{n,\mathbf{k}}$ along the conduction (CB) and (d,e) valence bands (VB) computed at $k = \Gamma, \mathrm{X}$ respectively. The black solid line indicates the center of mass of the electron wave, while the dashed-dotted line indicates the geometrical center of the unit cell. These **k**-points are indicated in red dots (diamonds) along the VB (CB) in panel (a).

## S3. DISTANCE FROM THE SCATTERING CENTER TO THE ELECTRODES

Here we show results for the crossed 8-ZGNRs with different GNR lengths, *i.e.*, different distances from the scattering center to the leads. We performed calculations for the same crossing with the same spin configuration ($\boxed{\uparrow\uparrow}$) and compare the spin densities to that corresponding to the perfect (periodic) ribbon solution, *i.e.*, uncoupled ribbons. To do so we plot in real space the difference between the local magnetization, defined as

$$m_i = \langle n_{i\uparrow} \rangle - \langle n_{i\downarrow} \rangle \,, \tag{S3}$$

for the self-consistent solution of the full device calculation and the local magnetization corresponding to the periodic ribbons, $m_i^0$.

In order to preserve the bulk nature for the electrodes, there must be a sufficient distance separating the scattering center from the leads. However, the highly localized Coulomb repulsion term seems to prevent the spin density of the device from being affected by this size effect as Fig. S5 shows that the spin polarization of the coupled ribbons is essentially unaffected by the position of the electrodes. In other words, the inter-GNR coupling induces changes in the electronic structure only in the near vicinity to the crossing.

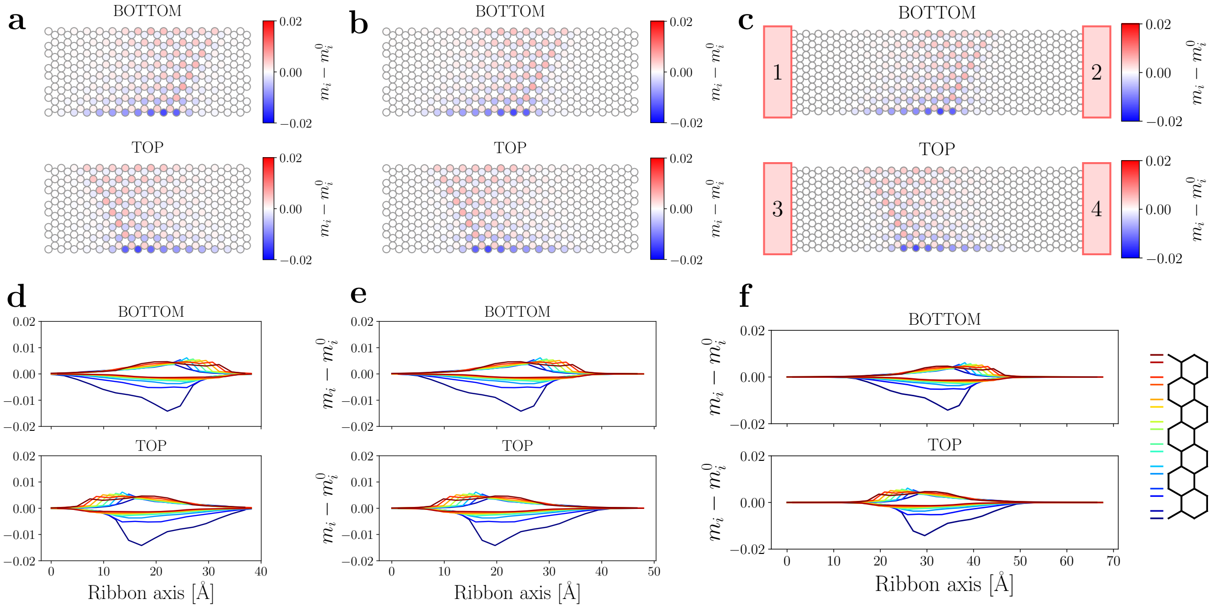


FIG. S5. Convergence study with respect to the size of the device region for AB-stacked 8-ZGNRs in the $\boxed{\uparrow\uparrow}$ configuration. (a-c) Difference between the calculated spin polarization for the 4-terminal device ($m_i$) and the spin polarization for decoupled ribbons ($m_i^0$) plotted in real space for different device sizes. We compare three cases, (a) one with a repetition of 16 ($\sim$ 38 Å), (b) another with 20 ($\sim$ 48 Å) and the last one with (c) 28 ($\sim$ 68 Å) ZGNR unit cells. The latter corresponds to the size of the device shown in the main text. (d-f) Profile of $m_i - m_i^0$ along the ribbon axis for different positions across the perpendicular direction (confinement direction). The legend on the left side indicates the transverse position of each profile.

## S4. ALL INEQUIVALENT SPIN CONFIGURATIONS AND TRANSMISSION CURVES FOR AB- AND AA-STACKINGS

Here we show all the unique spin configurations for AA- and AB-stacked 8-ZGNRs and the corresponding transmission and reflection probabilities for each spin component. We also list the electronic energy according to Eq. (S2) of each configuration. As mentioned in the main text, each spin configuration for this open quantum system is found by fixing spin density distribution of the 4 electrodes, leading to $2^4/2 = 8$ unique solutions to the imposed boundary conditions (excluding the trivial global inversion of the spin). To show these solutions we plot the difference between the spin densities for the $\uparrow$ and $\downarrow$ spin components, *i.e.*, $\langle n_\uparrow\rangle - \langle n_\downarrow\rangle$, in Figs. S6 and S7 for the AB- and AA-stacking, respectively.

In Tab. S1 we compare the relative electronic energies for the AA- and AB-stacked devices with the 8 unique spin-configurations (a-h) that arise from imposing the spin-densities in the electrodes.

| | **a** $\boxed{\uparrow\downarrow}$ | **b** $\boxed{\uparrow\uparrow}$ | **c** | **d** | **e** | **f** | **g** | **h** |
|---|---|---|---|---|---|---|---|---|
| **AB** | 0.000 | 0.082 | 0.387 | 0.398 | 0.202 | 0.202 | 0.203 | 0.203 |
| **AA** | 0.583 | 0.425 | 0.847 | 0.939 | 0.623 | 0.623 | 0.622 | 0.622 |

TABLE S1. Electronic energies $E_{\mathrm{tot}}$ according to Eq. (S2) for different spin configurations of the AB- (Fig. S6) and AA-stacked (Fig. S7) crossed 8-ZGNRs devices. The energies (in eV) are compared to the configuration of minimum energy corresponding to AB-stacked $\boxed{\uparrow\downarrow}$ in Fig. S6(a).

The first observation is that we find the AA-stacked devices to have larger electronic energy than the AB-stacked ones for all spin configurations (see Tab. S1). This result is in line with other results of this kind [8]. The second observation is that the ground state is the configuration with antiferromagnetic (AFM) alignment between layers, *i.e.*, the atoms that lie one on top of the other have opposite spin index, in line with results published in Ref. [9]. On the other hand, some of the spin configurations involve the presence of domain walls (grain boundaries), if the spin densities of the electrodes belonging to the same ribbon are inverted.

We observe that for configurations that have a single grain boundary, the domain wall moves along the ribbons to leave the scattering area (crossing) with the spin density distri-

bution that corresponds to the ground state configuration [cf. Figs. S6 and S7]. For instance, for the AB-stacked device, the grain boundary in Fig. S6(e-h) moves along the ribbons to leave the crossing with the spin density distribution of Fig. S6(a). Similarly, for the AA-stacked devices, the grain boundary moves along the ribbons to leave the crossing with the spin density distribution of Fig. S7(b). We find that, for the two cases without grain boundaries, the spin configuration of each ribbon deviates very little from that corresponding to the perfect (translationally invariant) 8-ZGNR, showing the weak coupling between them.

On the other hand, Fig. S8 and Fig. S9 shows the transmission and reflection probabilities for the AB- and AA-stacked devices with the different possible spin distributions. As it can be seen in these figures, and following the argument and discussion from the main text, the only systems that have $T_{ij}^{\sigma} \neq T_{ij}^{\bar{\sigma}}$ are those that only display black symmetry axes (break the symmetry between the spin indices). The transmission probability is computed as mentioned in the main text, while the reflection probability can be computed by subtracting the total outgoing transmission probability to the number of channels/modes existing at a certain energy, $M_{\alpha}$,

$$R_{\alpha}^{\sigma} = M_{\alpha}^{\sigma} - \sum_{\beta \neq \alpha} T_{\alpha\beta}^{\sigma}. \tag{S4}$$

We observe that both $R_1^s$ and $T_{14}^s$ are zero for energies lying in the single-band energy region for both stackings and all spin configurations, according to the unpolarized case [10].

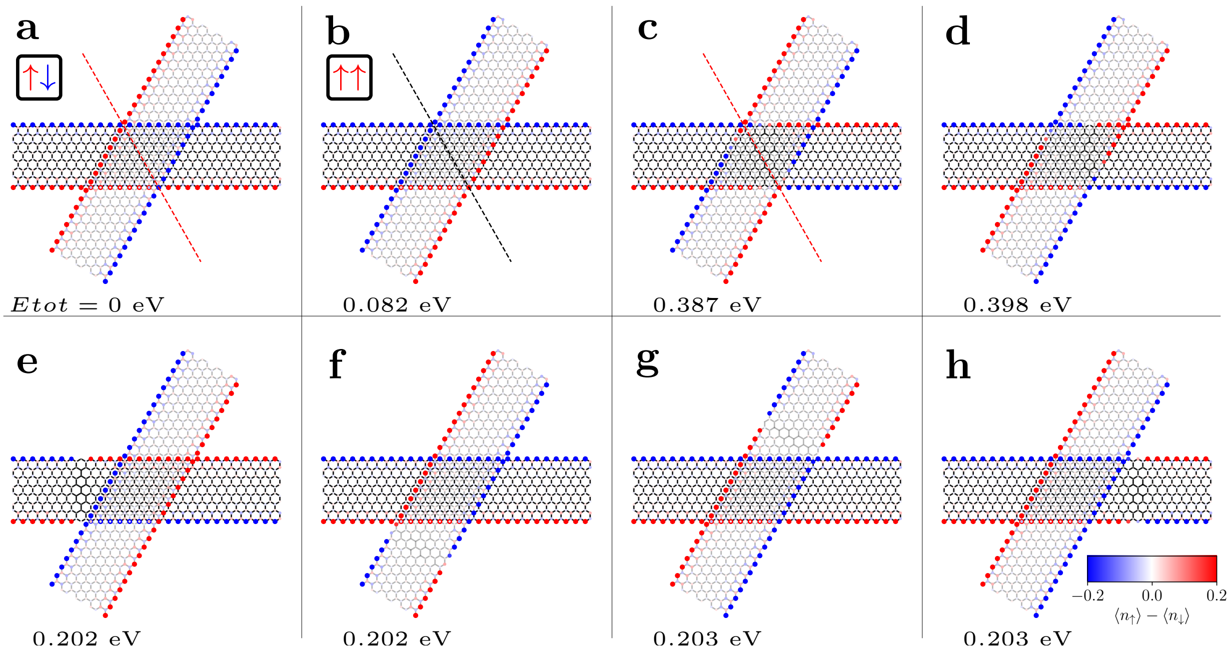


FIG. S6. Spin configurations for the AB-stacked 8-ZGNRs. The electronic energy $E_{\text{tot}}$ (in eV) of each configuration (relative to AB-stacked $\boxed{\uparrow\downarrow}$ in panel a) is noted in the bottom left corner in each panel. Red and black dashed lines indicate the symmetry axes.

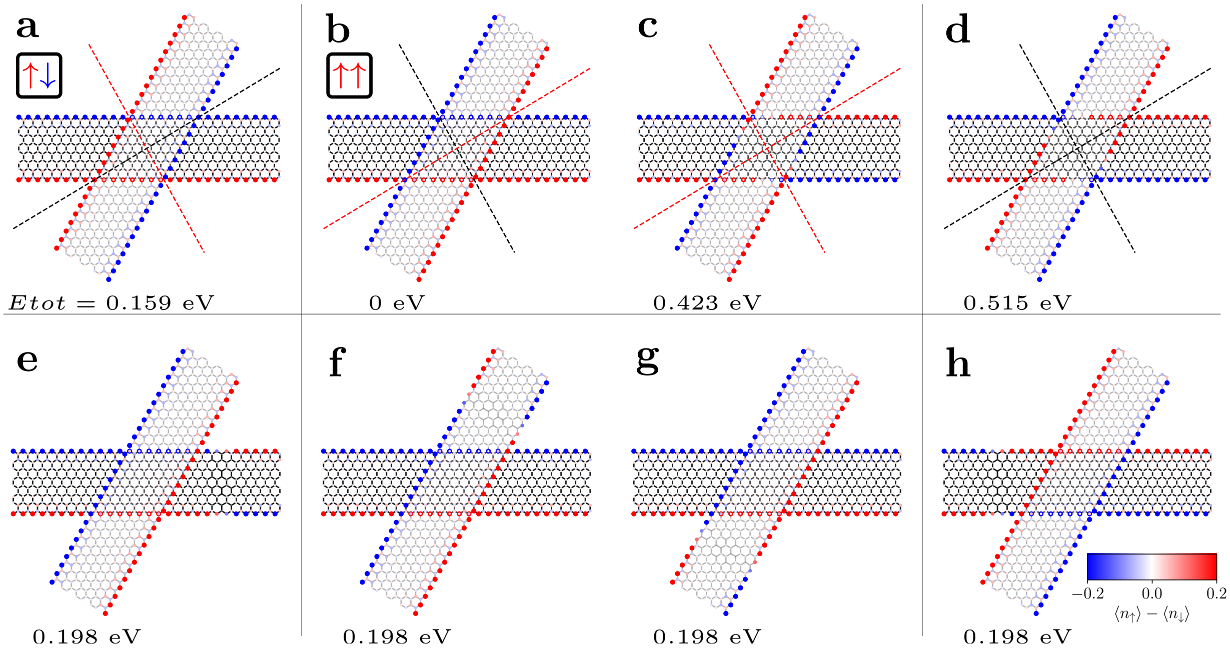


FIG. S7. As Fig. S6 but for the the AA-stacked 8-ZGNRs. The electronic energy $E_{\mathrm{tot}}$ (in eV) of each configuration (relative to AA-stacked $\boxed{\uparrow\uparrow}$ in panel b) is noted in the bottom left corner in each panel.

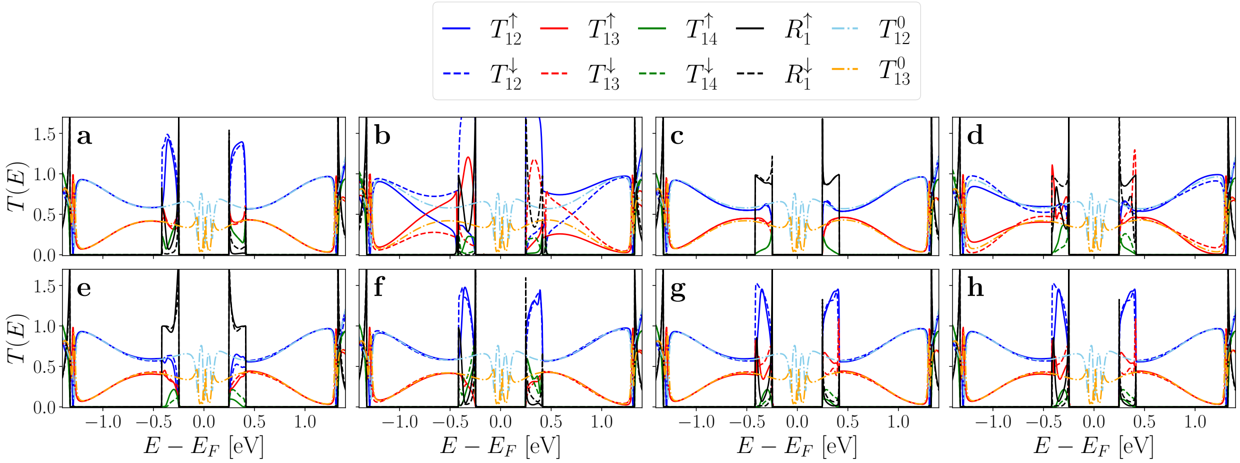


FIG. S8. Transmission and reflection probabilities per spin channel for the AB-stacked 8-ZGNRs shown in Fig. S6. $T^0_{12}$ and $T^0_{13}$ are the transmission probabilities between terminals $1 \rightarrow 2$ and $1 \rightarrow 3$ for the unpolarized device.

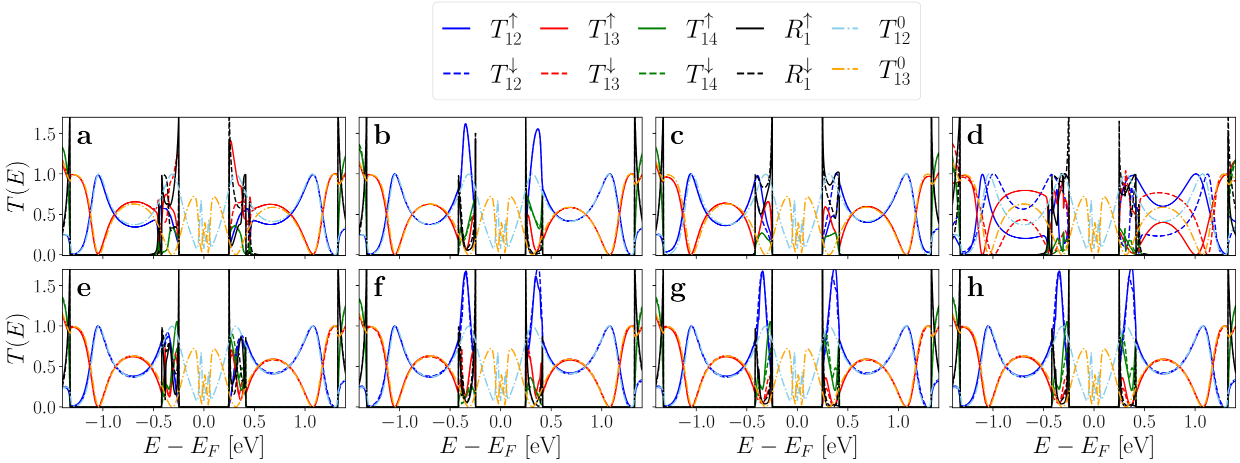


FIG. S9. As Fig. S8 but for the AA-stacked 8-ZGNRs shown in Fig. S7.

## S5. ELECTRONIC TOTAL ENERGY AND MAGNETIZATION

Fig. S10 shows the electronic part of the total energy of each device compared to the energy of the uncoupled system, $E_0$, as a function of the translation of the on top ribbon with respect to the bottom one starting with the geometry of the AB-stacked device. This energy can be understood as a binding energy between the ribbons. We note that this energy lacks some contributions that are not taken into account in this approximation, *e.g.*, the change in the Van der Waals forces as the two ribbons are translated with respect to each other which determines the precise inter-GNR separation, etc. Here, the geometrical distortion is only encoded through the Slater-Koster parametrization [10].

As mentioned above, the closest stackings to the AB pattern lie in a global minimum. The AA-stacking is a local minimum but more energetic than the AB-stacking. One interesting result is that the plots Fig. S10(a,b) are very similar, showing that the largest contribution to the electronic energy comes from the geometry and that the relative spin density distribution of the ribbons plays a minor role in this physical quantity.

Fig. S10(c,d) show the sum of local *magnetization changes* induced by the inter-GNR interaction, defined as $\sum_i |m_i| - |m_i^0|$. This shows that the magnetization of the device is always lower than that corresponding to the uncoupled ribbons. This last statement makes sense since the effect of the hopping amplitude between the GNRs goes "against" the localization of the electrons, and thus the local magnetization of the system. Therefore the local magnetization of the coupled ribbons will be lower than the magnetization of the uncoupled ribbons, especially in the coupled area. Fig. S10(c,d) also shows that for the configurations with FM inter-layer coupling (AB in Fig. S6b and AA in Fig. S7a, *i.e.*, the atoms that are vertically aligned have equal spin indices), the magnetization decreases more with respect to the perfect 8-ZGNR than configurations with AFM inter-layer coupling (AB in Fig. S6a and AA in Fig. S7b, *i.e.*, the atoms that are vertically aligned have opposite spin indices).

In panels Fig. S10(e,f) we show the maximum backscattering for configurations $\boxed{\uparrow\downarrow}$ and $\boxed{\uparrow\uparrow}$ as a function of the translation of the on-top ribbon with respect to the other one. We hereby see that the low reflection is general for the crossed ZGNRs.

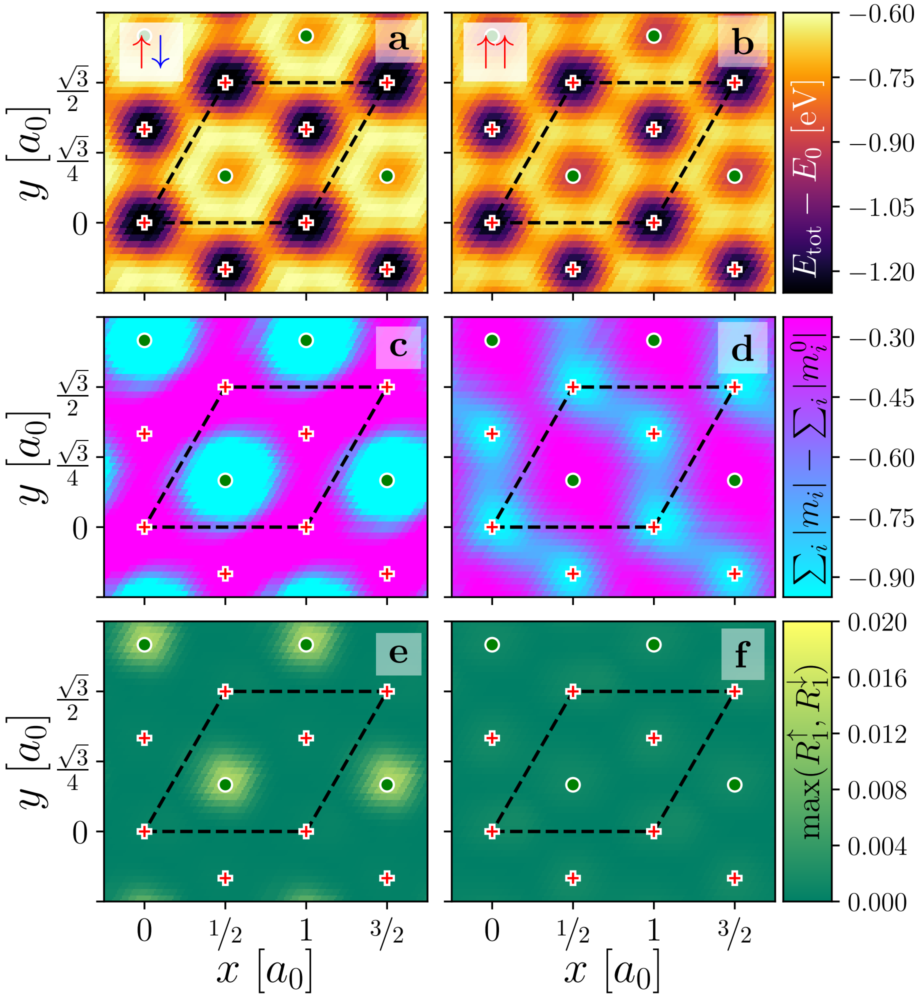


FIG. S10. (a,b) Electronic part of the total energy $E_{\mathrm{tot}}$ relative to the energy of the uncoupled system $E_0$, (c,d) sum of the absolute value of the magnetization $\sum_i |m_i|$ compared to the uncoupled system $\sum_i |m_i^0|$, and (e,f) maximum backscattering into terminal 1 as function of the translation of the top ribbon with respect to the bottom one for the two possible spin configurations $\boxed{\uparrow\uparrow}$ and $\boxed{\uparrow\downarrow}$, respectively. The dashed parallelogram corresponds to the primitive cell of the problem. Red crosses and green circles indicate the AB- and AA-stacking, respectively.

## S6. FIGURE OF MERIT

Fig. S11 shows the quality of the beam splitting or mirror effect per spin channel in the junctions, following the idea of [10], in a figure of merit defined as

$$\mathrm{FM} = e^{-20\lambda} \tanh\left[\frac{1}{20}\left(\frac{1}{|\tau-1|} - \frac{1}{|\tau-1/2|}\right)\right], \tag{S5}$$

that was firstly used and defined in the reference from above (the parameters $\lambda, \tau$ and their definition can be found there). Black areas show where the device behaves as a good beam splitter ($T_{12}^s \sim T_{13}^s \sim 0.5$). Red areas would show where the device behaves as a good mirror ($T_{13}^s \sim 1$), however the device is not wide enough to show this behavior (see ref. [10]). White areas indicate devices with almost perfect transmission ($T_{12}^s \sim 1$, since losses ($R^\sigma + T_{14}^s$) are less than 2% for all geometries) that are not of interest for our purposes.

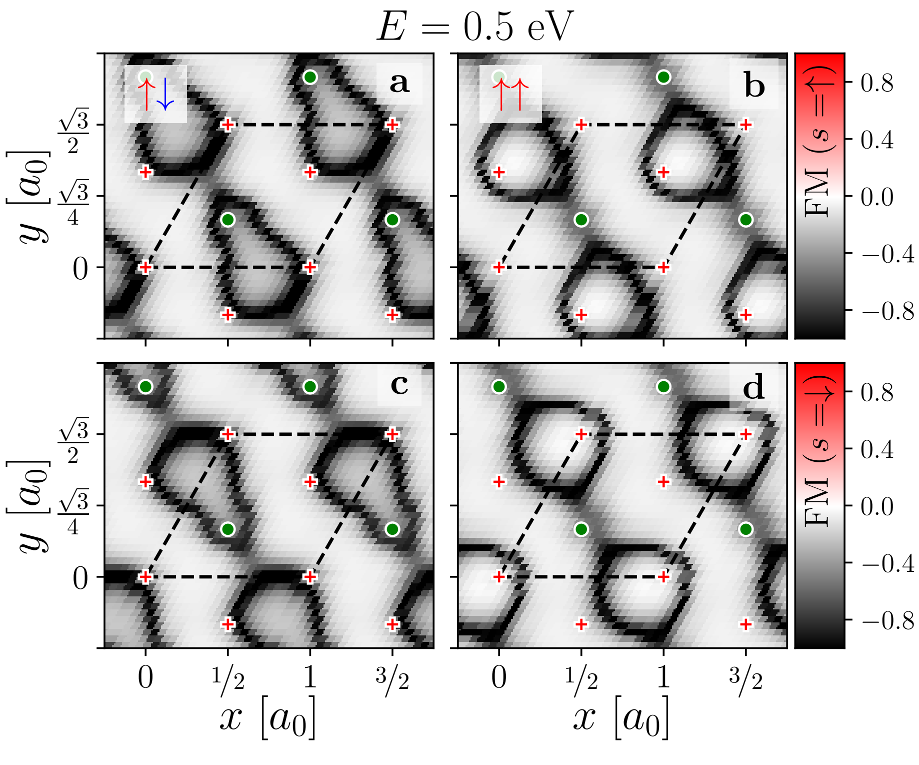


FIG. S11. (a,b) [(c,d)] Figure of merit (FM) for $\sigma = \uparrow$ [$\sigma = \downarrow$] as function of the translation of the top ribbon along the graphene periodicity vectors $\mathbf{a}_1$, $\mathbf{a}_2$ with respect to the bottom one for the two possible spin configurations ($\boxed{\uparrow\uparrow}$ and $\boxed{\uparrow\downarrow}$, respectively). Red crosses and green circles indicate the AB- and AA-stacking, respectively.

## S7. SPIN POLARIZATION FOR ELECTRONS AT OTHER ENERGY VALUES

In the main text we show the scattering states (spectral density of states) for an incoming electron with an energy of $E \sim 0.5$ eV for the AB-stacking four-terminal device. However, the polarization in the transport properties is an energy dependent quantity (as seen for instance in Fig. 2 of the main text). Therefore, for completeness we show in Fig. S12 the spectral density of states for $E \sim 1.0, -0.5, -1.0$ eV. One interesting observation is that panels (b,e) have opposite spin orientation at the edges of the ribbon with respect to panels (c,f). This can be understood from Fig. S4, where the center of mass of the waves changes sign (goes to zero) between $-0.5\,(+0.5)$ and $-1.0\,(+1.0)$ eV for the VB (CB).

Additionally we also show in Fig. S13 the polarization and the figure of merit for an incoming electron with energy $E \sim 0.5$ eV.

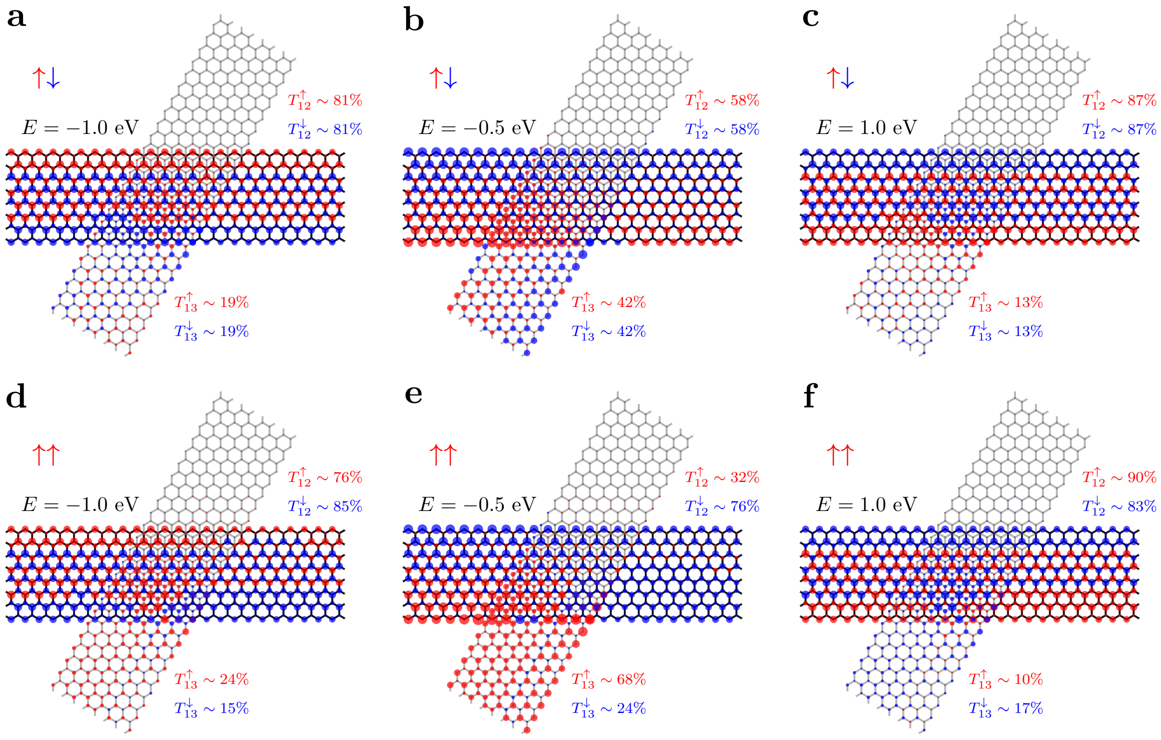


FIG. S12. Scattering states $\mathbf{A} = \mathbf{A}_{\uparrow} + \mathbf{A}_{\downarrow}$ for the (a-c) $\boxed{\uparrow\downarrow}$ and (d-f) $\boxed{\uparrow\uparrow}$ spin configuration computed at $E = -1.0$, $E = -0.5$, and $E = 1.0$ eV (electrons incoming from the left electrode 1). The dominant spin on each site at this energy is shown in red for up-spins and in blue for down-spins.

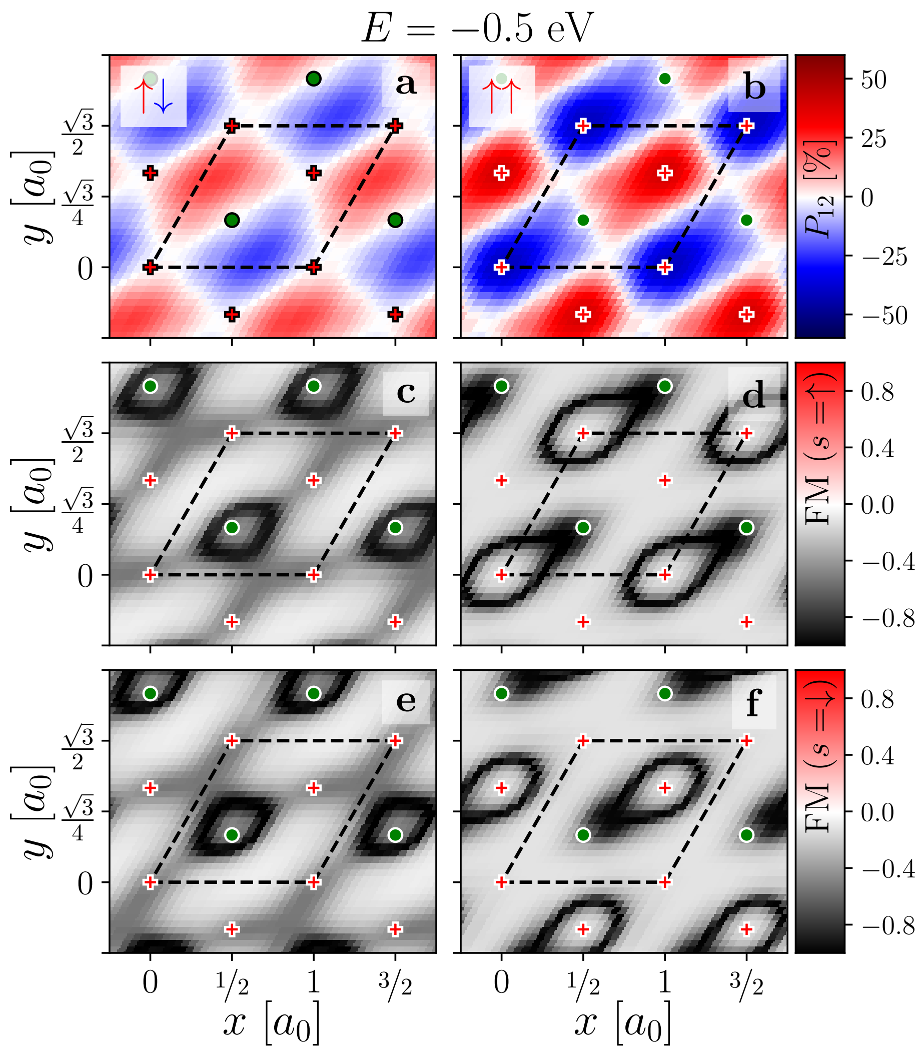


FIG. S13. (a,b) Polarization for an electron incoming from terminal 1 and outgoing in terminal 2 and (c,d) [(e,f)] figure of merit (FM) for $\sigma = \uparrow$ [$\sigma = \downarrow$] as function of the translation of the top ribbon along the graphene periodicity vectors $\mathbf{a}_1$, $\mathbf{a}_2$ with respect to the bottom one for the two possible spin configurations ($\boxed{\uparrow\uparrow}$ and $\boxed{\uparrow\downarrow}$, respectively) obtained at $E = -0.5$ eV. Red crosses and green circles indicate the AB- and AA-stacking, respectively.

## S8. ROLE OF RIBBON WIDTH

In this section we compute the spin polarization distribution and transmission and reflection probabilities as a function of the electron energy for different ribbon widths for the same crossing and spin configuration (AB-$\boxed{\uparrow\uparrow}$). We see that the different transport behavior for the two different spin channels is general for this crossing. On the other hand, we see that the inter-transmission probability ($T^s_{13}$) grows with the ribbon width, while the opposite behavior is found for the intra-transmission probability ($T^s_{12}$). Furthermore, losses ($R^s_1 + T^s_{14}$) remain absent independently of the width of the ribbon. These results are in line with the transport properties found for the unpolarized case [cf. Ref [10]].

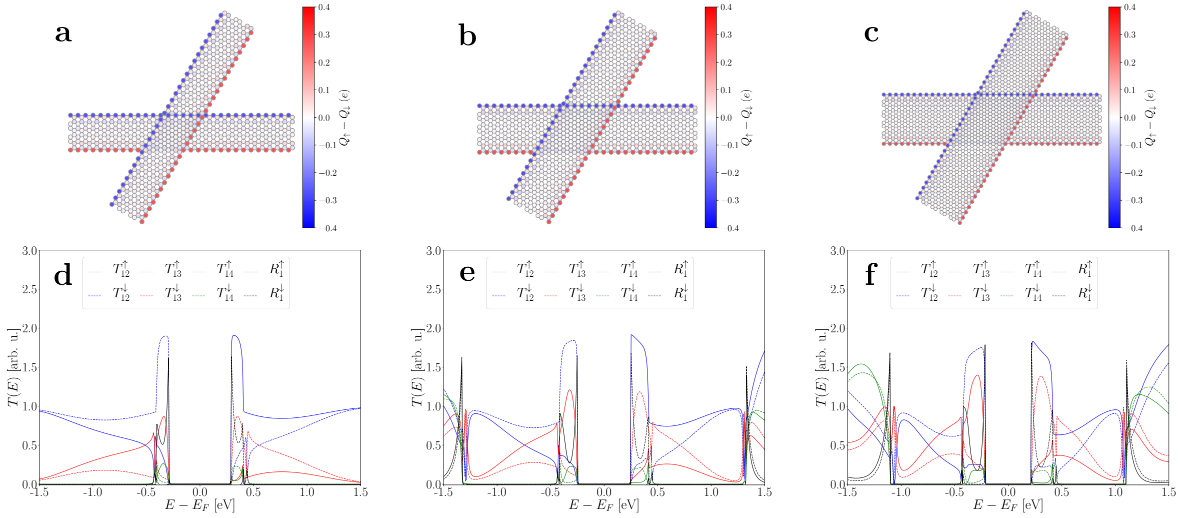


FIG. S14. Transmission coefficients for different ribbon widths. (a-c) Spin polarization for the 4-terminal device formed of two AB-stacked crossed 6-ZGNRs, 8-ZGNRs and 10-ZGNRs, respectively. (d-f) Transmission and reflection probabilities for an incoming electron from terminal 1 for the 6-ZGNRs, 8-ZGNRs and 10-ZGNRs device, respectively.

## S9. INDEPENDENT-SCATTERERS APPROXIMATION

To test the independent-scatterers approximation used in the main text (Fig. 4), where we consider each crossing as if it was independent from the others, we chose an array of 3 crossings. For simplicity we consider the unpolarized case although these results can be extrapolated to the polarized device since reflection is absent for this case too. In Fig. S15 we compare the exact transmission probabilities obtained for the full device with TBtrans [4] with the same transmission probabilities obtained within the independent-scatterers approximation (Eqs. (S6-S12)). This approximation would be exact if one obtained the overall transmission probabilities by coherently combining the scattering matrices of the successive sections using the Feynman paths [11]. Given the fact that there is no reflection for electrons with energies in the single-channel energy region there is no interference between the incoming waves and the reflected ones. Thus, in our approximation we only take the first term of the Feynman path (direct multiplication of the corresponding scattering matrices). Naming the single crossing transmission probabilities with lowercase letters $t_{12}$, $t_{13}$ and $t_{14}$, we obtain the transmission probabilities for the full device (named with upper case $T_{ij}$) as following:

$$T_{12} = t_{12}^3 \tag{S6}$$

$$T_{13} = t_{13} \tag{S7}$$

$$T_{14} = t_{14} \tag{S8}$$

$$T_{15} = t_{12}t_{13} \tag{S9}$$

$$T_{16} = t_{12}t_{14} \tag{S10}$$

$$T_{17} = t_{12}^2 t_{13} \tag{S11}$$

$$T_{18} = t_{12}^2 t_{14}. \tag{S12}$$

We observe in Fig. S15 that the independent-scatterers approximation is practically exact in the single-channel energy region (where there is only one available mode). The reason for this excellent agreement, as mentioned above, comes from the fact that there is no reflection for these energy values, therefore the interference terms between the backscattered waves disappear. This is not the case outside the single-channel energy region.

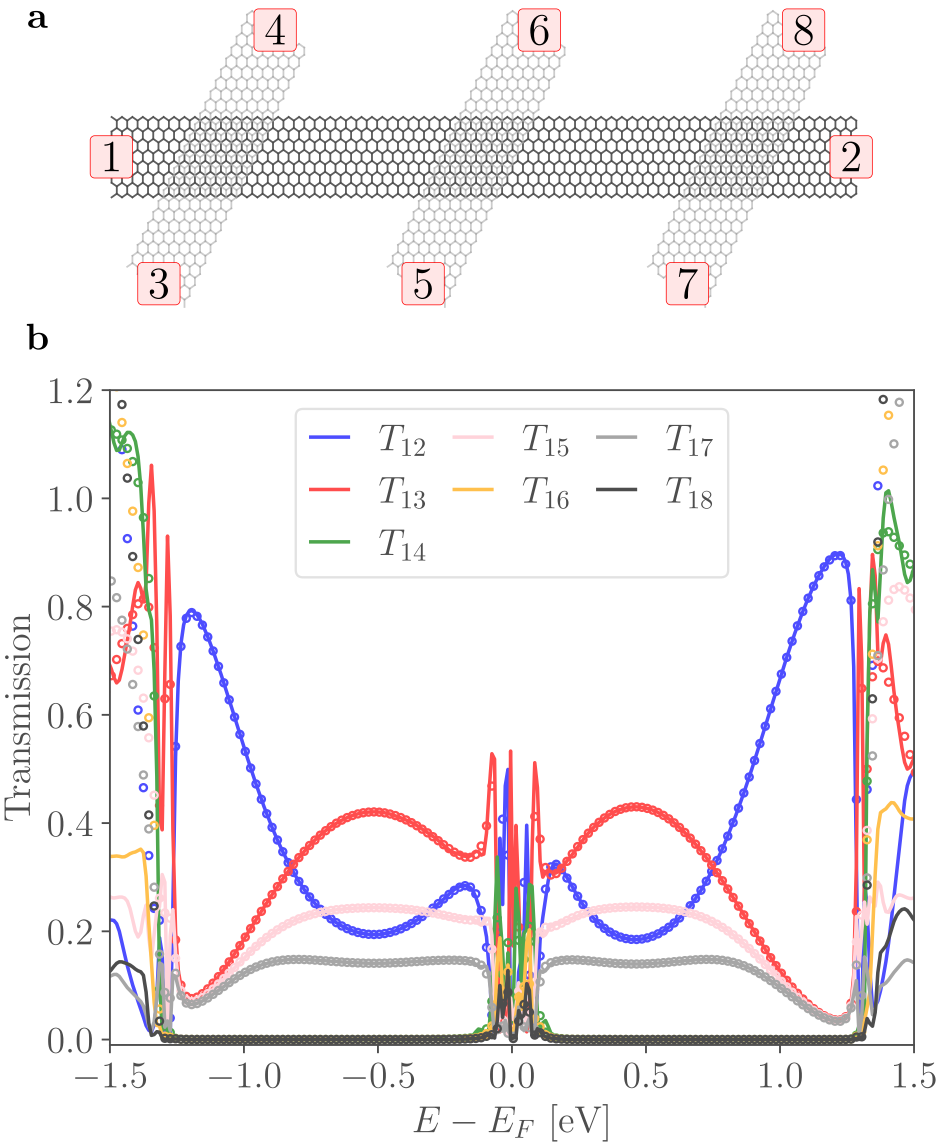


FIG. S15. (a) Geometry of the device with three consecutive crossings. All 8 terminals are indicated in red squares. (b) Transmission probabilities between the different pairs of terminals for an incoming electron in terminal 1 as a function of the electron energy. Solid lines represent the transmission probability for the full device, while open circles represent the obtained transmission probability using the independent-scatterers approximation.

## S10. AVERAGED TRANSMISSION PROBABILITIES

In this section we compute the averaged transmission probabilities, calculated as $\bar{T}_{ij} = (T_{ij}^{\uparrow} + T_{ij}^{\downarrow})/2$, for both spin configurations $\boxed{\uparrow\uparrow}$ and $\boxed{\uparrow\downarrow}$ compared to the unpolarized case in Fig. S16. By comparing these results and the ones shown in the main text, it can be seen that while the spin-averaged transmission of the device reproduces our earlier results [10] (*i.e.*, it is affected very little by inclusion of the mean-field Coulomb interaction), we find a strong spin-dependence of the transmission, something that is completely absent in the non-interacting case.

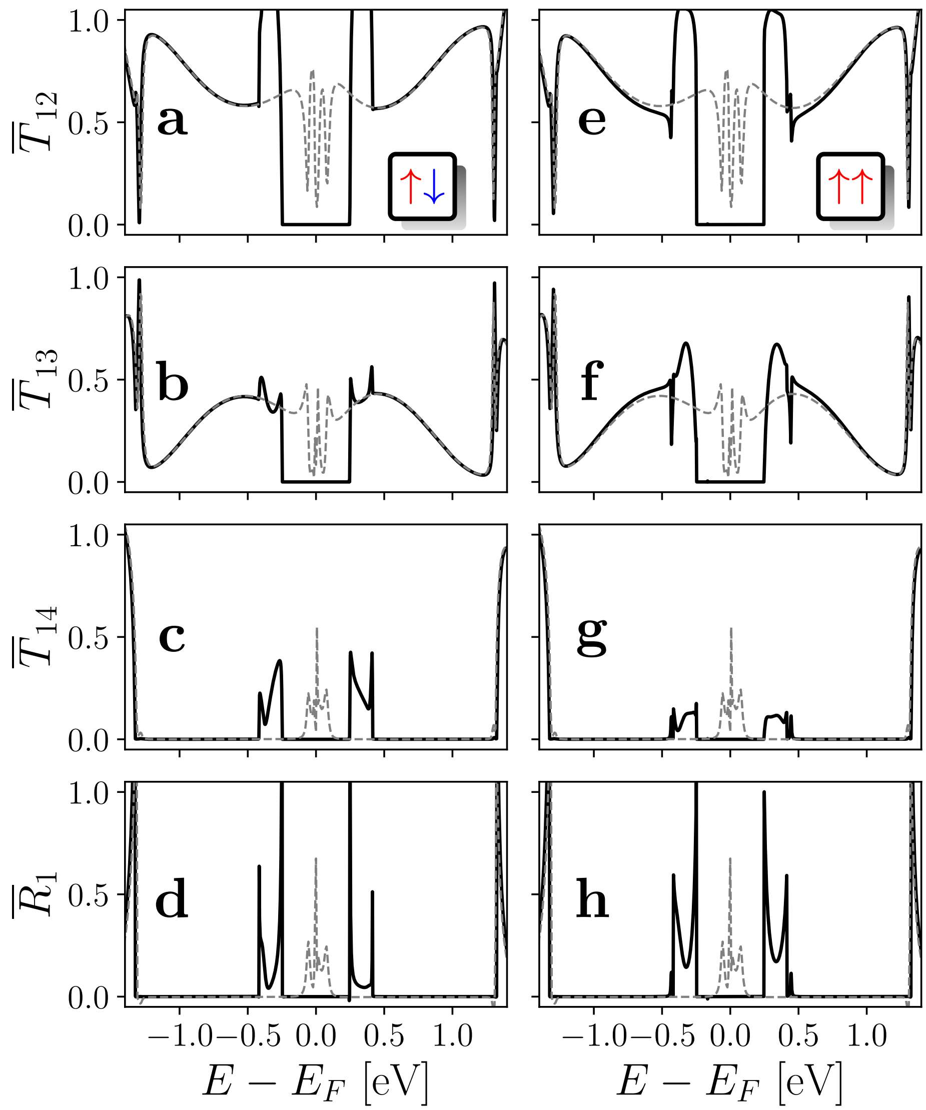


FIG. S16. Black solid lines stand for $\bar{T}_{ij} = (T_{ij}^{\uparrow} + T_{ij}^{\downarrow})/2$ while the gray dashed lines stand for the unpolarized transmission probabilities.

## S11. ROLE OF CROSSING GEOMETRY FOR THE SPIN-POLARIZING TRANSPORT EFFECT

We note that there are some experimental challenges to realize the proposed devices, for example to control the stacking registry and the twist angle. These parameters were already assessed in Ref. [10] for unpolarized devices, showing that the beam splitting effect remained largely unaffected by these perturbations, however in that analysis the Coulomb repulsion was not included. For this reason, in this section we study the behavior of the spin transport properties of the crossed ZGNRs for different spin configurations ($\boxed{\uparrow\uparrow}$ and $\boxed{\uparrow\downarrow}$), intersection angles (within 55-65°), and stacking registries at the crossing. In Fig. S17 we show both $P_{12}$ and the maximum reflection probability $R_1^>$ as a function of the in-plane translation of the top ribbon with respect to the lower one for different intersection angles and the two spin configurations $\boxed{\uparrow\downarrow}$ and $\boxed{\uparrow\uparrow}$. Here we observe that both $\boxed{\uparrow\downarrow}$ and $\boxed{\uparrow\uparrow}$ configurations still show spin-polarized current generally for different angles and translations. Even in the case of $\boxed{\uparrow\downarrow}$, which diminishes its polarization to $P_{12} \leq 10\%$ for angles $\theta > 64°$, we find that this effect is reverted for $E = -0.5$ eV, where the polarization grows with the angle and only diminishes for $\theta < 56°$ (not shown here). We also observe that backscattering remains rather small for crossed ZGNRs regardless the stacking configuration. This result extends to the whole single-mode energy region (not shown here).

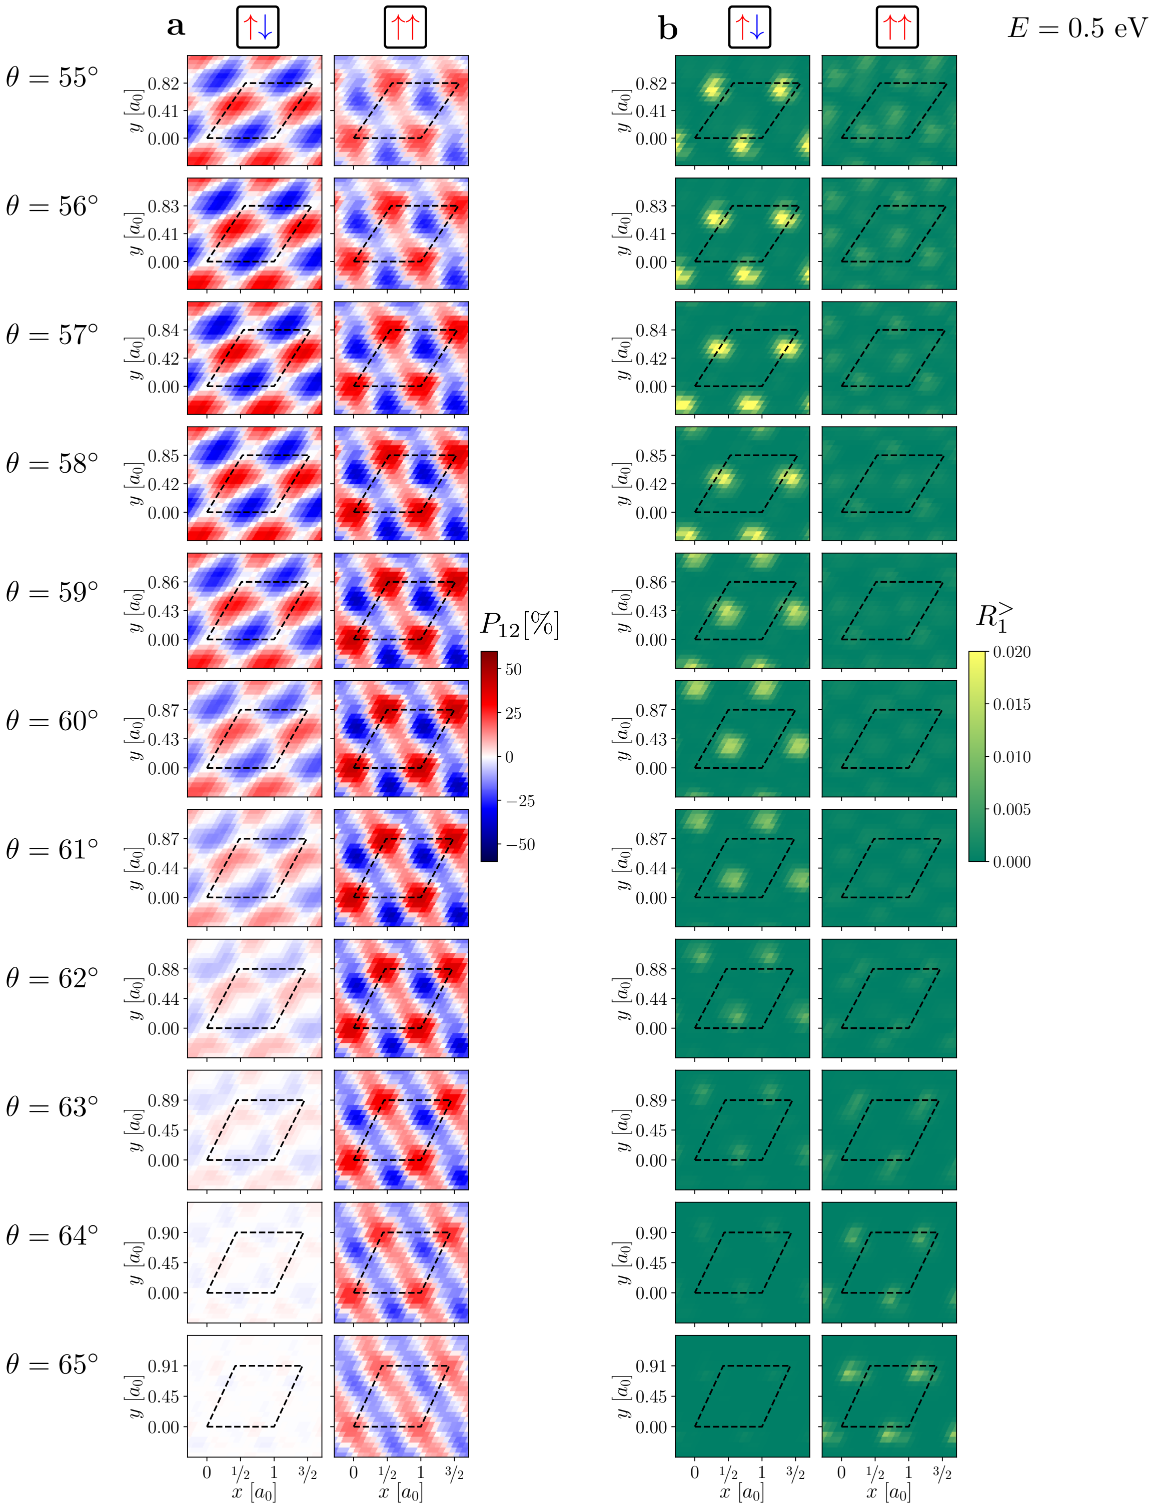


FIG. S17. (a) Spin polarization $P_{12}$ of the current from electrode 1 to 2 and (b) maximum of reflection probability, $R_1^> = \max(R_1^\uparrow, R_1^\downarrow)$ as function of in-plane translations of one ribbon with respect to the other for the $\boxed{\uparrow\uparrow}$ and $\boxed{\uparrow\downarrow}$ spin configurations at different intersection angles. The electron energy is fixed at $E = 0.5$ eV. The unit cell, defined by the lattice vectors of the two ribbons (forming the angle $\theta$), is indicated by the black parallelogram.

## S12. STATISTICAL ANALYSIS OF RANDOM ARRAY DEVICES

In this section we provide a description of the statistical analysis behind the results presented in Fig. 4(b) of the main text. We begin with a derivation of the analytic expression of the average absolute spin polarization of arrays $\langle|\overline{P_{12}}|\rangle$.

Starting from Eq. (2) of the main text for the polarization $P_{12}$ of a single junction, we can express the polarization $\overline{P_{12}}$ of an array of $N$ junctions as

$$\overline{P_{12}}(N) = \frac{1 - e^{\overline{\lambda}(N)}}{1 + e^{\overline{\lambda}(N)}}, \tag{S13}$$

where

$$\overline{\lambda}(N) = \sum_{i=1}^{N} \lambda_i, \tag{S14}$$

$$\lambda_i = \ln \frac{T_{12}^{\downarrow}(i)}{T_{12}^{\uparrow}(i)}. \tag{S15}$$

Assuming independent and identical distribution (iid) of the configuration (angle and displacement) of each crossing, it follows from the multiplicative central limit theorem that the ratio $e^{\overline{\lambda}(N)}$ follows a *log-normal* distribution with parameters $\overline{\mu} = \mu N$ and $\overline{w} = w\sqrt{N}$, where $\mu$ and $w^2$ are the mean and variance, respectively, of $\lambda$ for an individual crossing.

In the unbiased (worst) case, $\mu = 0$, as for the present systems, this allows us to write the *absolute value* averages

$$\langle|\overline{\lambda}(N)|\rangle = \int_{-\infty}^{\infty} ds\ |s|\ \mathcal{N}(s, 0, \overline{w}^2) = \overline{w}\sqrt{\frac{2}{\pi}} = w\sqrt{\frac{2N}{\pi}} = \Lambda\sqrt{N}, \tag{S16}$$

$$\begin{aligned}\langle e^{-|\overline{\lambda}(N)|}\rangle &= \int_{-\infty}^{\infty} ds\ e^{-|s|}\ \mathcal{N}(s, 0, \overline{w}^2) = e^{\overline{w}^2/2}\ \text{erfc}\left[\frac{\overline{w}}{\sqrt{2}}\right] = e^{w^2 N/2}\ \text{erfc}\left[w\sqrt{\frac{N}{2}}\right] \\ &= e^{\pi\Lambda^2 N/4}\ \text{erfc}\left[\Lambda\frac{\sqrt{\pi N}}{2}\right],\end{aligned} \tag{S17}$$

$$\langle|\overline{P_{12}}(N)|\rangle = \int_{-\infty}^{\infty} ds \left|\frac{1 - e^s}{1 + e^s}\right| \mathcal{N}(s, 0, \overline{w}^2), \tag{S18}$$

where $\langle\cdots\rangle$ denotes the statistical average, $\Lambda \equiv \langle|\lambda_1|\rangle$ the average for a single junction, and $\mathcal{N}(s, \overline{\mu}, \overline{w}^2)$ the normal distribution. Note that these expressions are only strictly relevant in our case for $N \to \infty$, where the use of the normal distribution is fully justified. Fig. S19

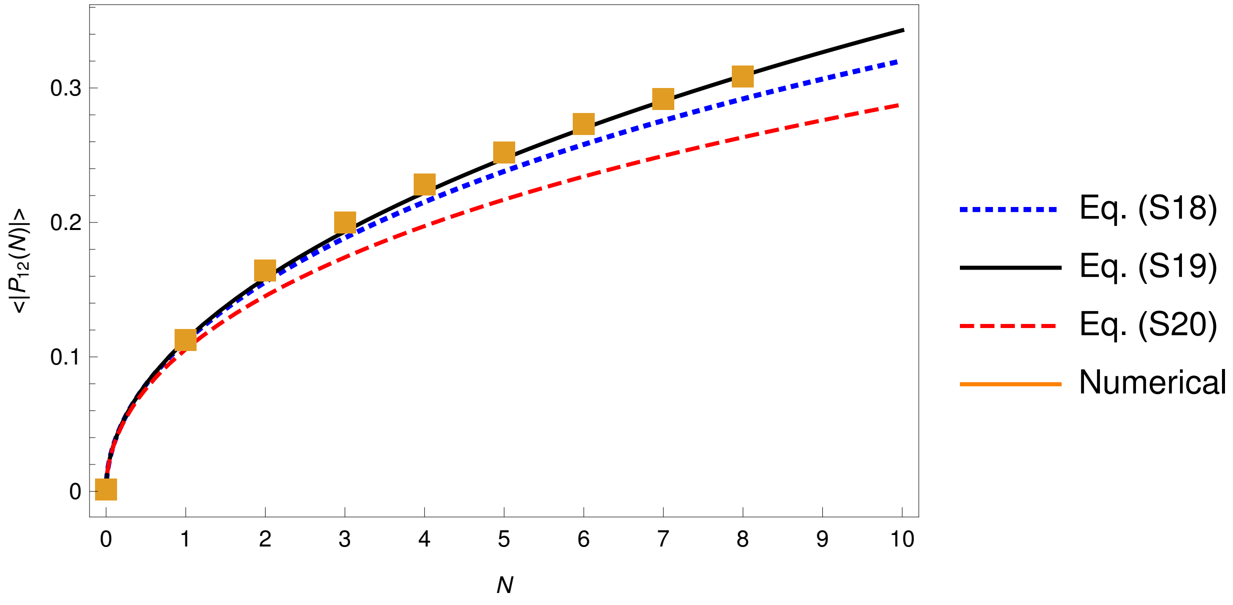


FIG. S18. Comparison of Eqs. (S18)-(S20) (blue, black and red lines, respectively) for the statistical average $\langle|\overline{P_{12}}(N)|\rangle$ against the direct numerical evaluation (orange squares) from the generated random data set, from which one also obtains the parameter $\Lambda \equiv \langle|\lambda_1|\rangle = 0.22602$.

below shows the actual convergence of the distribution for $\overline{\lambda}$ as $N$ increases.

From Eq. (S16) and Eq. (S17) we can write two approximate expressions for the average *absolute polarization*:

$$\langle|\overline{P_{12}}|\rangle \approx \frac{1 - e^{-\langle|\overline{\lambda}(N)|\rangle}}{1 + e^{-\langle|\overline{\lambda}(N)|\rangle}} = \frac{1 - e^{-\Lambda\sqrt{N}}}{1 + e^{-\Lambda\sqrt{N}}}, \tag{S19}$$

$$\langle|\overline{P_{12}}|\rangle \approx \frac{1 - \langle e^{-|\overline{\lambda}(N)|}\rangle}{1 + \langle e^{-|\overline{\lambda}(N)|}\rangle}. \tag{S20}$$

A comparison of the different statistical averages based on the assumption of a normal distribution is shown in Fig. S18 against the direct numerical evaluation of the average for the generated data set. The approach to 1 exponentially in $\sqrt{N}$ according to Eq. (S16) suggests the intuitive interpretation of the spin filtering mechanism in terms of 1D random walk as at each crossing a step $\lambda_i$ of random length and direction on the real line is added to $\overline{\lambda}$. Note that the approximation Eq. (S16) fits the curve for $\langle|P_{12}|\rangle$ surprisingly well. This is partially accidental and, as seen in Fig. S18, the fit is systematically worse for larger $N$ (as the variance of $\overline{\lambda}(N)$ increases).

Let us next turn to the actual statistical sampling procedure. The data set behind Fig. 4b in of the main text relies on an unbiased sampling of $10^7$ different spin-, intersection

angle, and translation configurations for each $N$ drawn from the actual realizations behind Fig. S17. The angle is sampled uniformly within the range $\theta \in [55^\circ, 65^\circ]$ in steps of $1^\circ$, while the translations are sampled over the unit cell on a $10 \times 10$ uniform grid. In Fig. S19 and Fig. S20 we show the histograms for the quantities $\overline{\lambda}(N)$ and $|\overline{P_{12}}|$. Our assumption of equal probability weight for all configurations is to keep things simple, although in reality the commensurate structures may be energetically favored. The main point of this statistical analysis is to show that a microscopic control over the individual crossings is not necessary to obtain a spin-polarizing array.

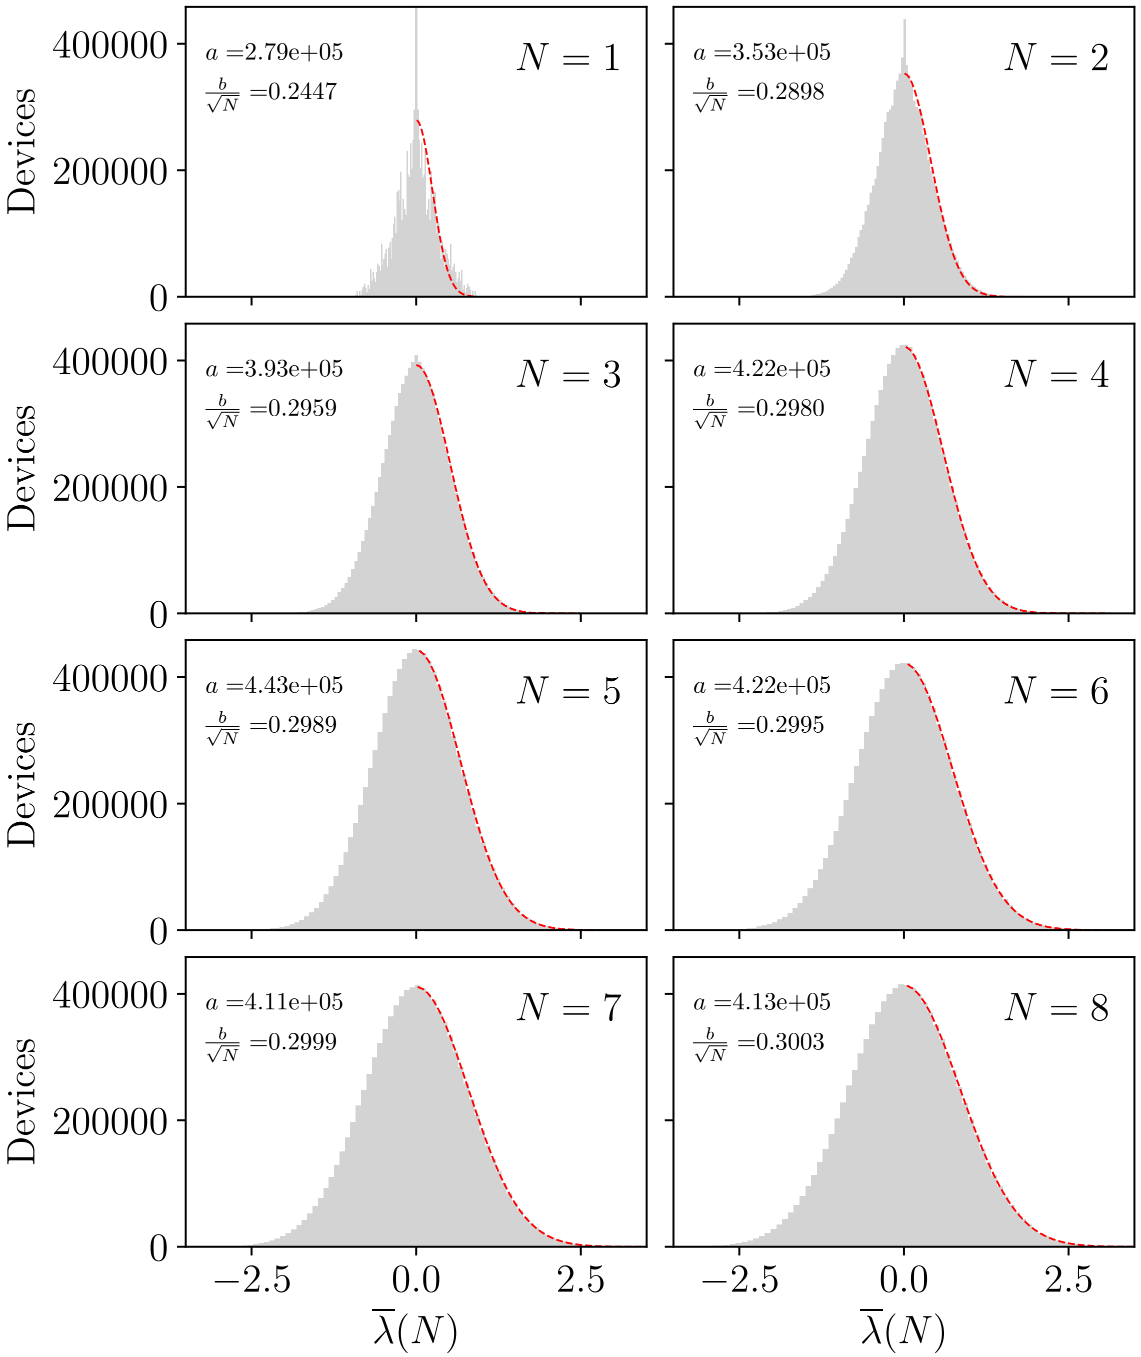


FIG. S19. Histogram of the distribution (100 bins) of $\overline{\lambda}(N)$ from $10^7$ random devices. The red dashed lines correspond to a Gaussian fitting $f(\overline{\lambda}) = a \exp\left(-\overline{\lambda}^2/2b^2\right)$, where the resulting fitting parameters $a, b$ are indicated in each panel.

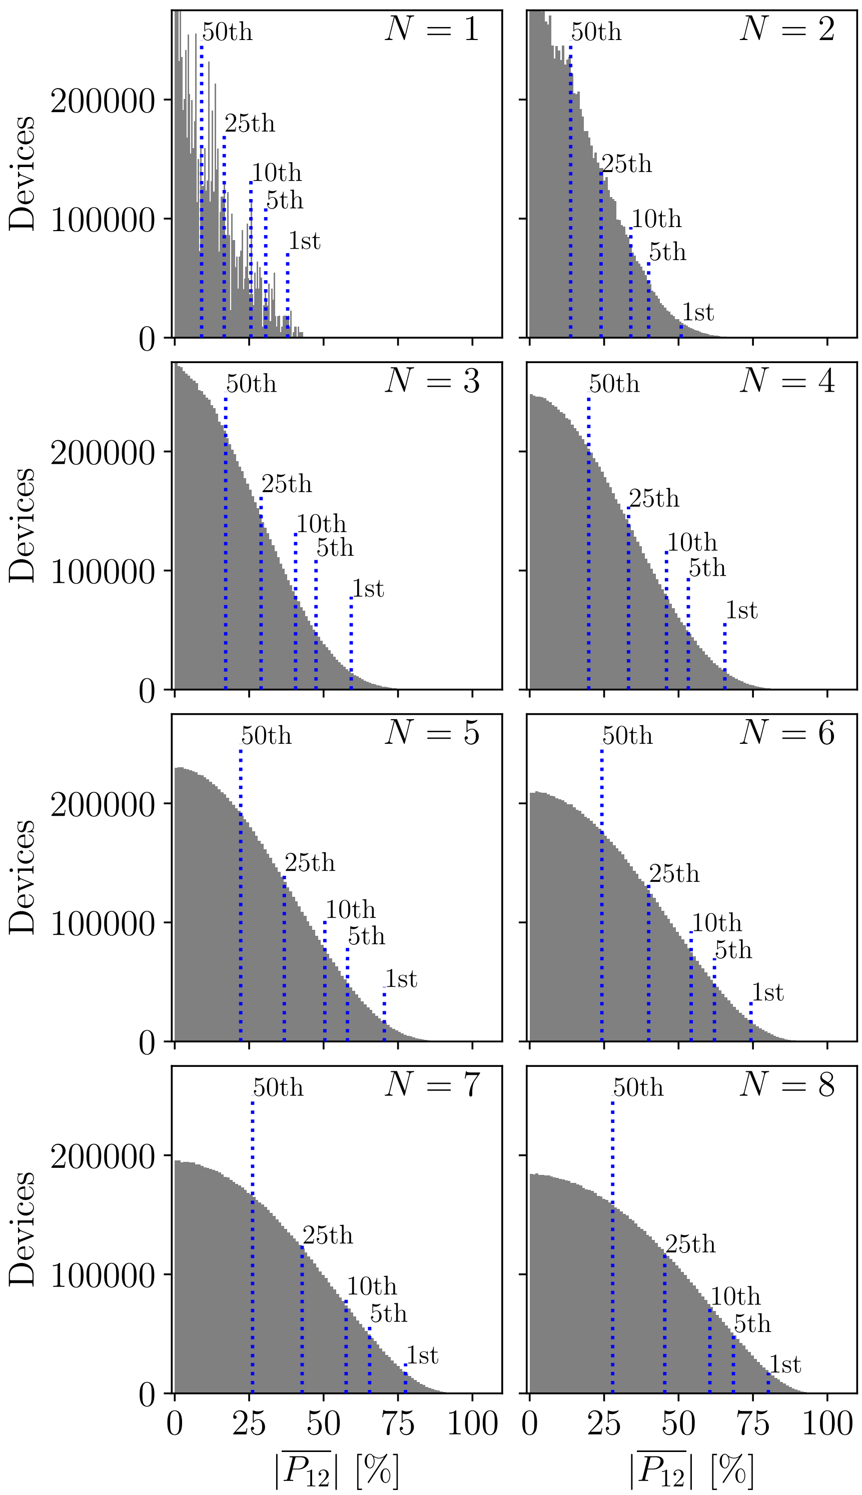


FIG. S20. Histogram of the distribution (100 bins) of $|\overline{P_{12}}|$ from $10^7$ random devices. The best (1, 5, 10, 25, 50)th percentiles are indicated with blue dotted lines in each panel.

## S13. A SPIN-POLARIZING BEAM SPLITTER WITH BEARDED GNRS

In this section we analyze the transport properties of intersecting bearded GNRs. The band structure and geometry of this structure is shown in Fig. S21. Although, to our knowledge, these systems have not yet been synthesized, we discuss these devices to complete our analysis on spin polarizing beam splitters formed by two crossed general GNRs. This type of GNRs are oriented along the zigzag direction but display different physical edges than ZGNRs. However, they present similar spin-polarized edge states as seen in Fig. S21. In Fig. S22 we plot both the self-consistent solutions $\boxed{\uparrow\uparrow}$ and $\boxed{\uparrow\downarrow}$ and the scattering states for this device, while in Fig. S23 we show the more detailed transmission probabilities for an incoming electron into terminal 1 as a function of the electronic energy. Figures S22 and S23 supports that both the beam splitting effect and the spin-polarizing scattering potential are general features of junctions with *edge-polarized GNRs*.

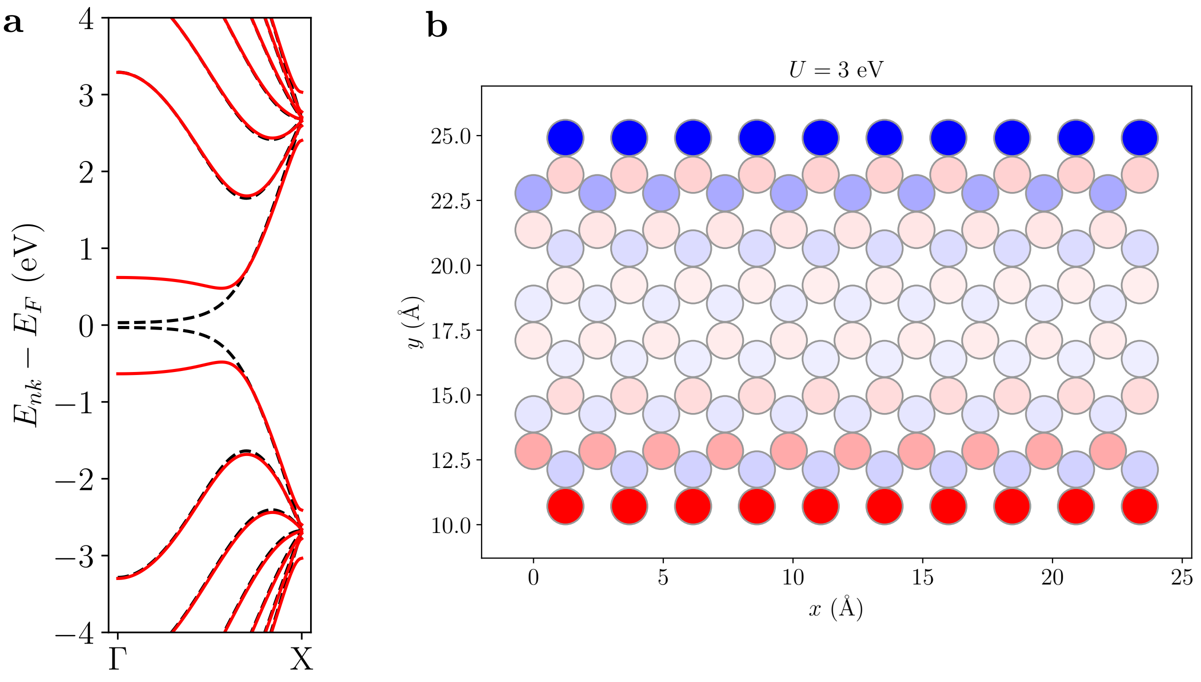


FIG. S21. (a) Band structure for the bearded GNR calculated with $U = 0$ (dashed black lines) and $U = 3$ eV (solid red lines). (b) Spin density for the periodic structure ($U = 3$ eV).

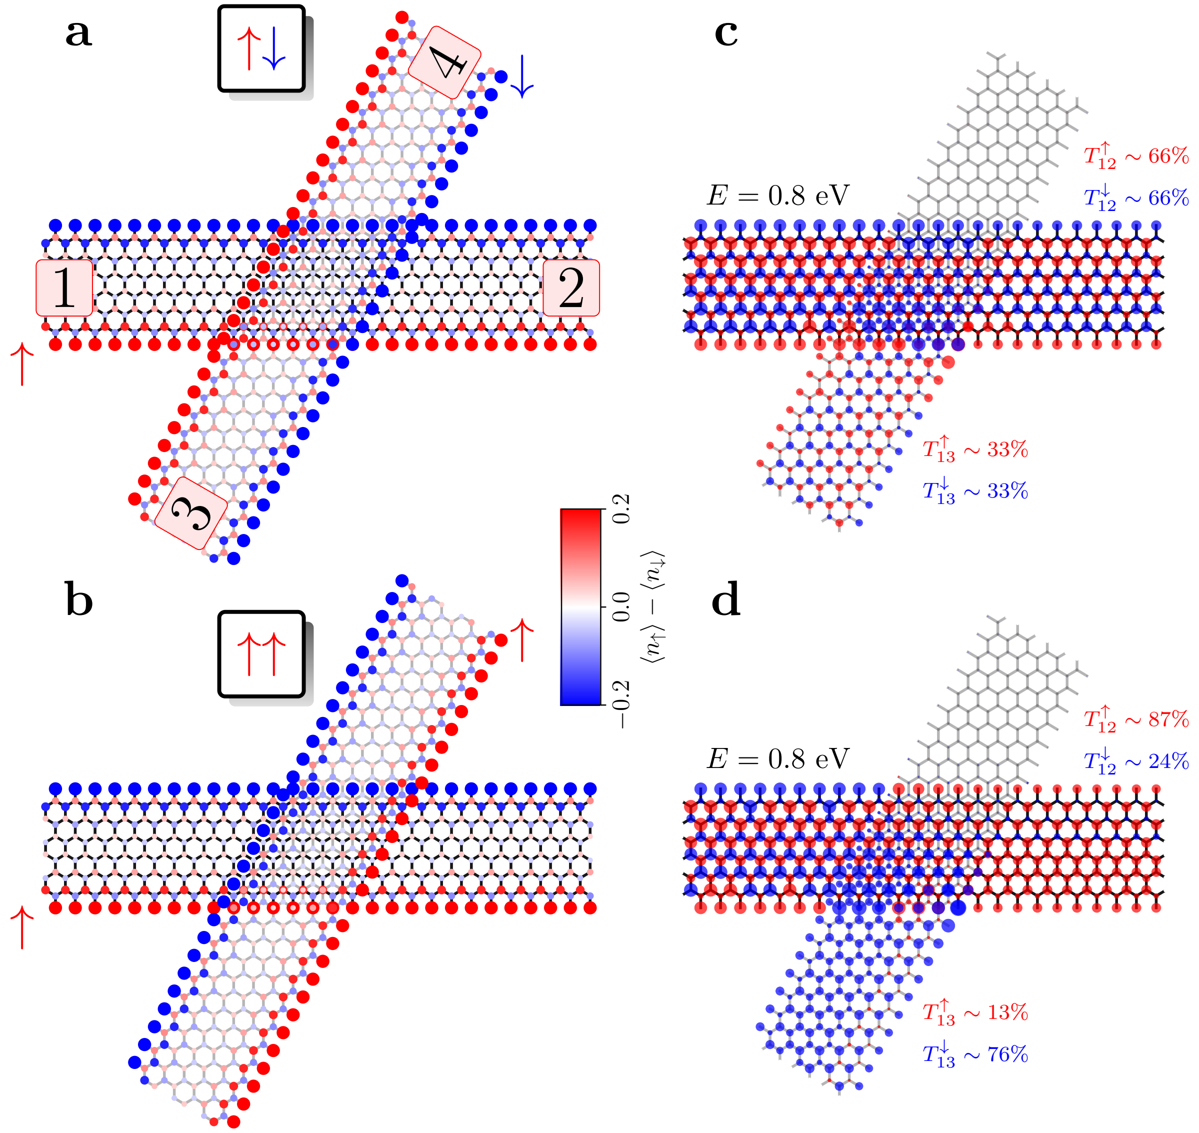


FIG. S22. (a,b) Spin density distribution for the crossed bearded-GNRs with an intersection angle of $\theta = 60°$. (c,d) Spin-resolved scattering states for an incoming electron from terminal 1 calculated at $E = 0.8$ eV. The dominant spin on each site at this energy is shown in red for up-spins and in blue for down-spins. The transmission probabilities $T^{\sigma}_{12}$ and $T^{\sigma}_{13}$ are annotated.

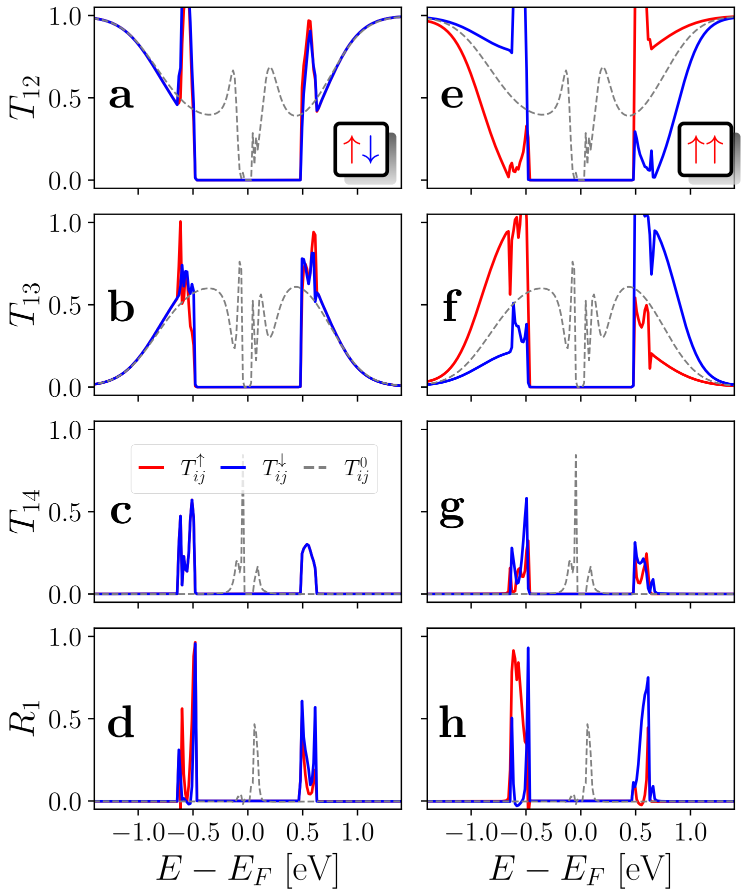


FIG. S23. Spin- and energy-resolved transmission probabilities $T_{12}$, $T_{13}$, $T_{14}$, and reflection $R_1$ for (a-d) the ↑↓ and (e-h) ↑↑ configurations. Electrons are injected from electrode 1. The red (blue) curves correspond to the up (down) spin components with $U = 3$ eV. For comparison, the corresponding calculations for the unpolarized case is indicated by dashed gray lines.

[1] H. Feldner, Z. Y. Meng, T. C. Lang, F. F. Assaad, S. Wessel, and A. Honecker, Phys. Rev. Lett. **106**, 226401 (2011).

[2] S. Sanz, N. Papior, M. Brandbyge, and T. Frederiksen, hubbard: v0.1.0 (2021).

[3] M. Brandbyge, J.-L. Mozos, P. Ordejón, J. Taylor, and K. Stokbro, Phys. Rev. B **65**, 165401 (2002).

[4] N. Papior, N. Lorente, T. Frederiksen, A. García, and M. Brandbyge, Comp. Phys. Commun. **212**, 8 (2017).

[5] M. P. L. Sancho, J. M. L. Sancho, J. M. L. Sancho, and J. Rubio, J. Phys. F: Met. Phys. **15**, 851 (1985).

[6] N. Papior, sisl: v0.11.0 (2021).

[7] T. Asano and J. Nakamura, ACS Omega **4**, 22035 (2019).

[8] E. Mostaani, N. D. Drummond, and V. I. Fal'ko, Phys. Rev. Lett. **115**, 115501 (2015).

[9] H. Lee, Y.-W. Son, N. Park, S. Han, and J. Yu, Phys. Rev. B **72**, 174431 (2005).

[10] S. Sanz, P. Brandimarte, G. Giedke, D. Sánchez-Portal, and T. Frederiksen, Phys. Rev. B **102**, 035436 (2020).

[11] M. Cahay, M. McLennan, and S. Datta, Phys. Rev. B **37**, 10125 (1988).
